# Supplementary material for: QDOT: Quantized Dot Product Kernel for Approximate High-Performance Computing
Source: arXiv:2105.00115 source file (2021-04-30)
Supplement: Supplementary file 1 [file appendix.tex]

%\clearpage
\appendix

\section{qdot: Toy Example}
\label{sec:appendixb}
%\textcolor{red}{(Update with different values of $\varepsilon$).} 
Let $\bm{x}, \bm{y} \in \mathbb{R}^4$ with $\bm{x} = [2^{27}, 2^{8}, 2^{-3}, 2^{20}]^{\intercal}$ and $\bm{y} = [2^{23}, 2^{-14}, 2^{7}, 2^{-3}]^{\intercal}$.
\iffalse %%%%%%%%%%%%%%%%%%%%%%
\begin{align}
    \bm{x} = \begin{bmatrix}
        2^{27} \\
        2^{8} \\
        2^{-3} \\
        2^{20}
    \end{bmatrix}
    \quad \text{and} \quad
    \bm{y} = \begin{bmatrix}
        2^{23} \\
        2^{-14} \\
        2^{7} \\
        2^{-3}
    \end{bmatrix},
\end{align}
\fi %%%%%%%%%%%%%%%%%%%%%%%%%%
Let \qdot \ tolerance be $\varepsilon = 2^{-34} \approx \texttt{5.8207661e-11}$. Suppose that the precision for $\bm{x}$ and $\bm{y}$ is \dpr. To use \textbf{qdot}, the first step is to determine the parameters that will yield approximation error bounded by $\varepsilon$. Following the details of Algorithm~\ref{alg:qdot-param}, the first step is to extract and sum the unbiased floating point exponents of $\bm{x}$ and $\bm{y}$ as follows
\begin{align}
\bm{e} 
&= \fl(\bm{x}) + \fl(\bm{y})
= [27, 8, -3, 20]^{\intercal} + [23, -14, 7, -3]^{\intercal}
= [50, -6, 4, 17]^{\intercal}
\end{align}
\iffalse %%%%%%%%%%%%%%%%%%%%%%
\begin{align}
\bm{e} 
&= \fl(\bm{x}) + \fl(\bm{y})
= \begin{bmatrix}
        27 \\
        8 \\
        -3 \\
        20
    \end{bmatrix} 
    + 
    \begin{bmatrix}
        23 \\
        -14 \\
        7 \\
        -3
    \end{bmatrix} 
= \begin{bmatrix}
        50 \\
        -6 \\
        4 \\
        17
    \end{bmatrix}.
\end{align}
\fi %%%%%%%%%%%%%%%%%%%%%%%%%%
Next, we identify the minimum and maximum values in $\bm{e}$ which yields $e_{\min} = -6$ and $e_{\max} = 50$. Next, sorting the elements of $\bm{e}$ in non-decreasing order yields $\bm{e} = [50, 17, 4, -6]^{\intercal}$.
\iffalse %%%%%%%%%%%%%%%%%%%%%%
\begin{align}
\bm{e} 
&= \begin{bmatrix}
        50 \\
        17 \\
        4 \\
        -6
    \end{bmatrix}.
\end{align}
\fi %%%%%%%%%%%%%%%%%%%%%%%%%%
Exact binning yields four nonempty bins with indices corresponding to the original ordering of the arrays $\bm{x}$ and $\bm{y}$ given by $B_{49,50} = \{ 1 \}$, $B_{16,17} = \{ 4 \}$, $B_{3,4} = \{ 3 \}$, and $B_{-7,-6} = \{ 2 \}$, with all other exact bins being the empty set. Computing the bin scores for each nonempty bin using (\ref{eq:bin-score-def}) with $\varepsilon = 2^{-34}$ %(since the inputs are assumed to be in \dpr \ precision) 
yields scores of 35, 2, -11, and -21. From the Precision function in (\ref{eq:precision-def}), we now have the precision for each bin to be $(B_{49,50}, \dpr)$, $(B_{16,17}, \hpr)$, $(B_{3,4}, \ppr)$, and $(B_{-7,-6}, \ppr)$. %At this point, the parameter selection algorithm is complete and we now use these parameters to compute the approximate kernel.

%Using $\bm{x}$, $\bm{y}$, and the identified parameters as inputs to Algorithm~\ref{alg:qdot-comp}, 
For computation we initialize two subvectors and perforate two components from computation. This ultimately yields a computation for \textbf{qdot} that looks like
\begin{align}
    \aunderbrace[l1r]{\strut 2^{27} * 2^{23} \strut}_{\strut \text{\dpr}}
    \ + \ \aunderbrace[l1r]{\strut 2^{8} * 2^{-14} \strut}_{\strut \text{\ppr}}
    \ + \ \aunderbrace[l1r]{\strut 2^{-3} * 2^{7} \strut}_{\strut \text{\ppr}}
    \ + \ \aunderbrace[l1r]{\strut 2^{20} * 2^{-3} \strut}_{\strut \text{\hpr}}.
\end{align}
As the value $2^{20}$ cannot be represented in \hpr \ precision, we highlight how rescaling is performed within \qdot \ in such an instance. First, the exponents are zeroed out in each component for the \hpr \ bin. Then the dot product for the entire bin is computed which in this instance is a single product. Finally, the resulting value is converted to \dpr \ to allow for rescaling to the correct value by multiplying by $2^{u_k}$, where $u_k$ is the maximum exponent value shared by all componentwise products in the bin. In this case, we multiply by $2^{17}$. While this process is trivial for this toy example, it is provided below for completeness:
\begin{align}
    \{ [2^{20}], [2^{-3}] \}
    &\xrightarrow[\text{(in \dpr)}]{\text{Zero exponents}} \{ [2^{0}], [2^{0}] \}
    \xrightarrow[\text{(in \hpr)}]{\text{Compute bin dot product}} 2^{0} \cdot 2^{0} = 2^0
    \xrightarrow[\text{(in \dpr)}]{\text{Rescale}} 2^{0} \cdot 2^{17} = 2^{17}.
\end{align}
Hence, \qdot \ yields $2^{50} + 2^{17}$ 
%. When compared to the full precision dot product, we now have a relative error of
which has a relative approximation error of
$\frac{2^4 + 2^{-6}}{2^{50} + 2^{17} + 2^4 + 2^{-6}} \approx \texttt{1.5e-14} < \varepsilon$.
